# Supplementary material for: Towards Learning Geometric Eigen-Lengths Crucial for Fitting Tasks
Source: arXiv:2312.15610 source file (2023-12-25)
Supplement: Supplementary file 1 [file 6_social.tex]

\section{Negative Social Impact}
Our work joins the initial efforts of eigen-length emergence in unsupervised learning settings with many other works along this direction.
There could be several bias in the data and training objectives, but this is a general concern shared by most works in this field. 
Our work may also share the controversial arguments with other works that the future AI agents may have the capability of thinking by themselves causing threats for human beings. 
However, the results demonstrated in our work are way far from that.
Other than these potential issues mentioned above, we do not see any other major concerns our work particularly introduces.
